# Supplementary material for: SIMCOPILOT: Evaluating Large Language Models for Copilot-Style Code Generation
Source: arXiv:2505.21514 source file (2025-05-21)
Supplement: Supplementary file 1 [file visual_support.tex]

\section{Visualization of Results}

\begin{figure}[h!]
	\centering
	\includegraphics[width=0.8\textwidth]{supplement/figs/group_by_ref_dist.png}
	\caption{Group by Reference Distribution}
	\label{fig:group_by_ref_dist}
\end{figure}

\begin{figure}[h!]
	\centering
	\includegraphics[width=0.8\textwidth]{supplement/figs/Comment_Dist_v2.png}
	\caption{Comment Distribution Version 2}
	\label{fig:comment_dist_v2}
\end{figure}

\begin{figure}[h!]
	\centering
	\includegraphics[width= \textwidth]{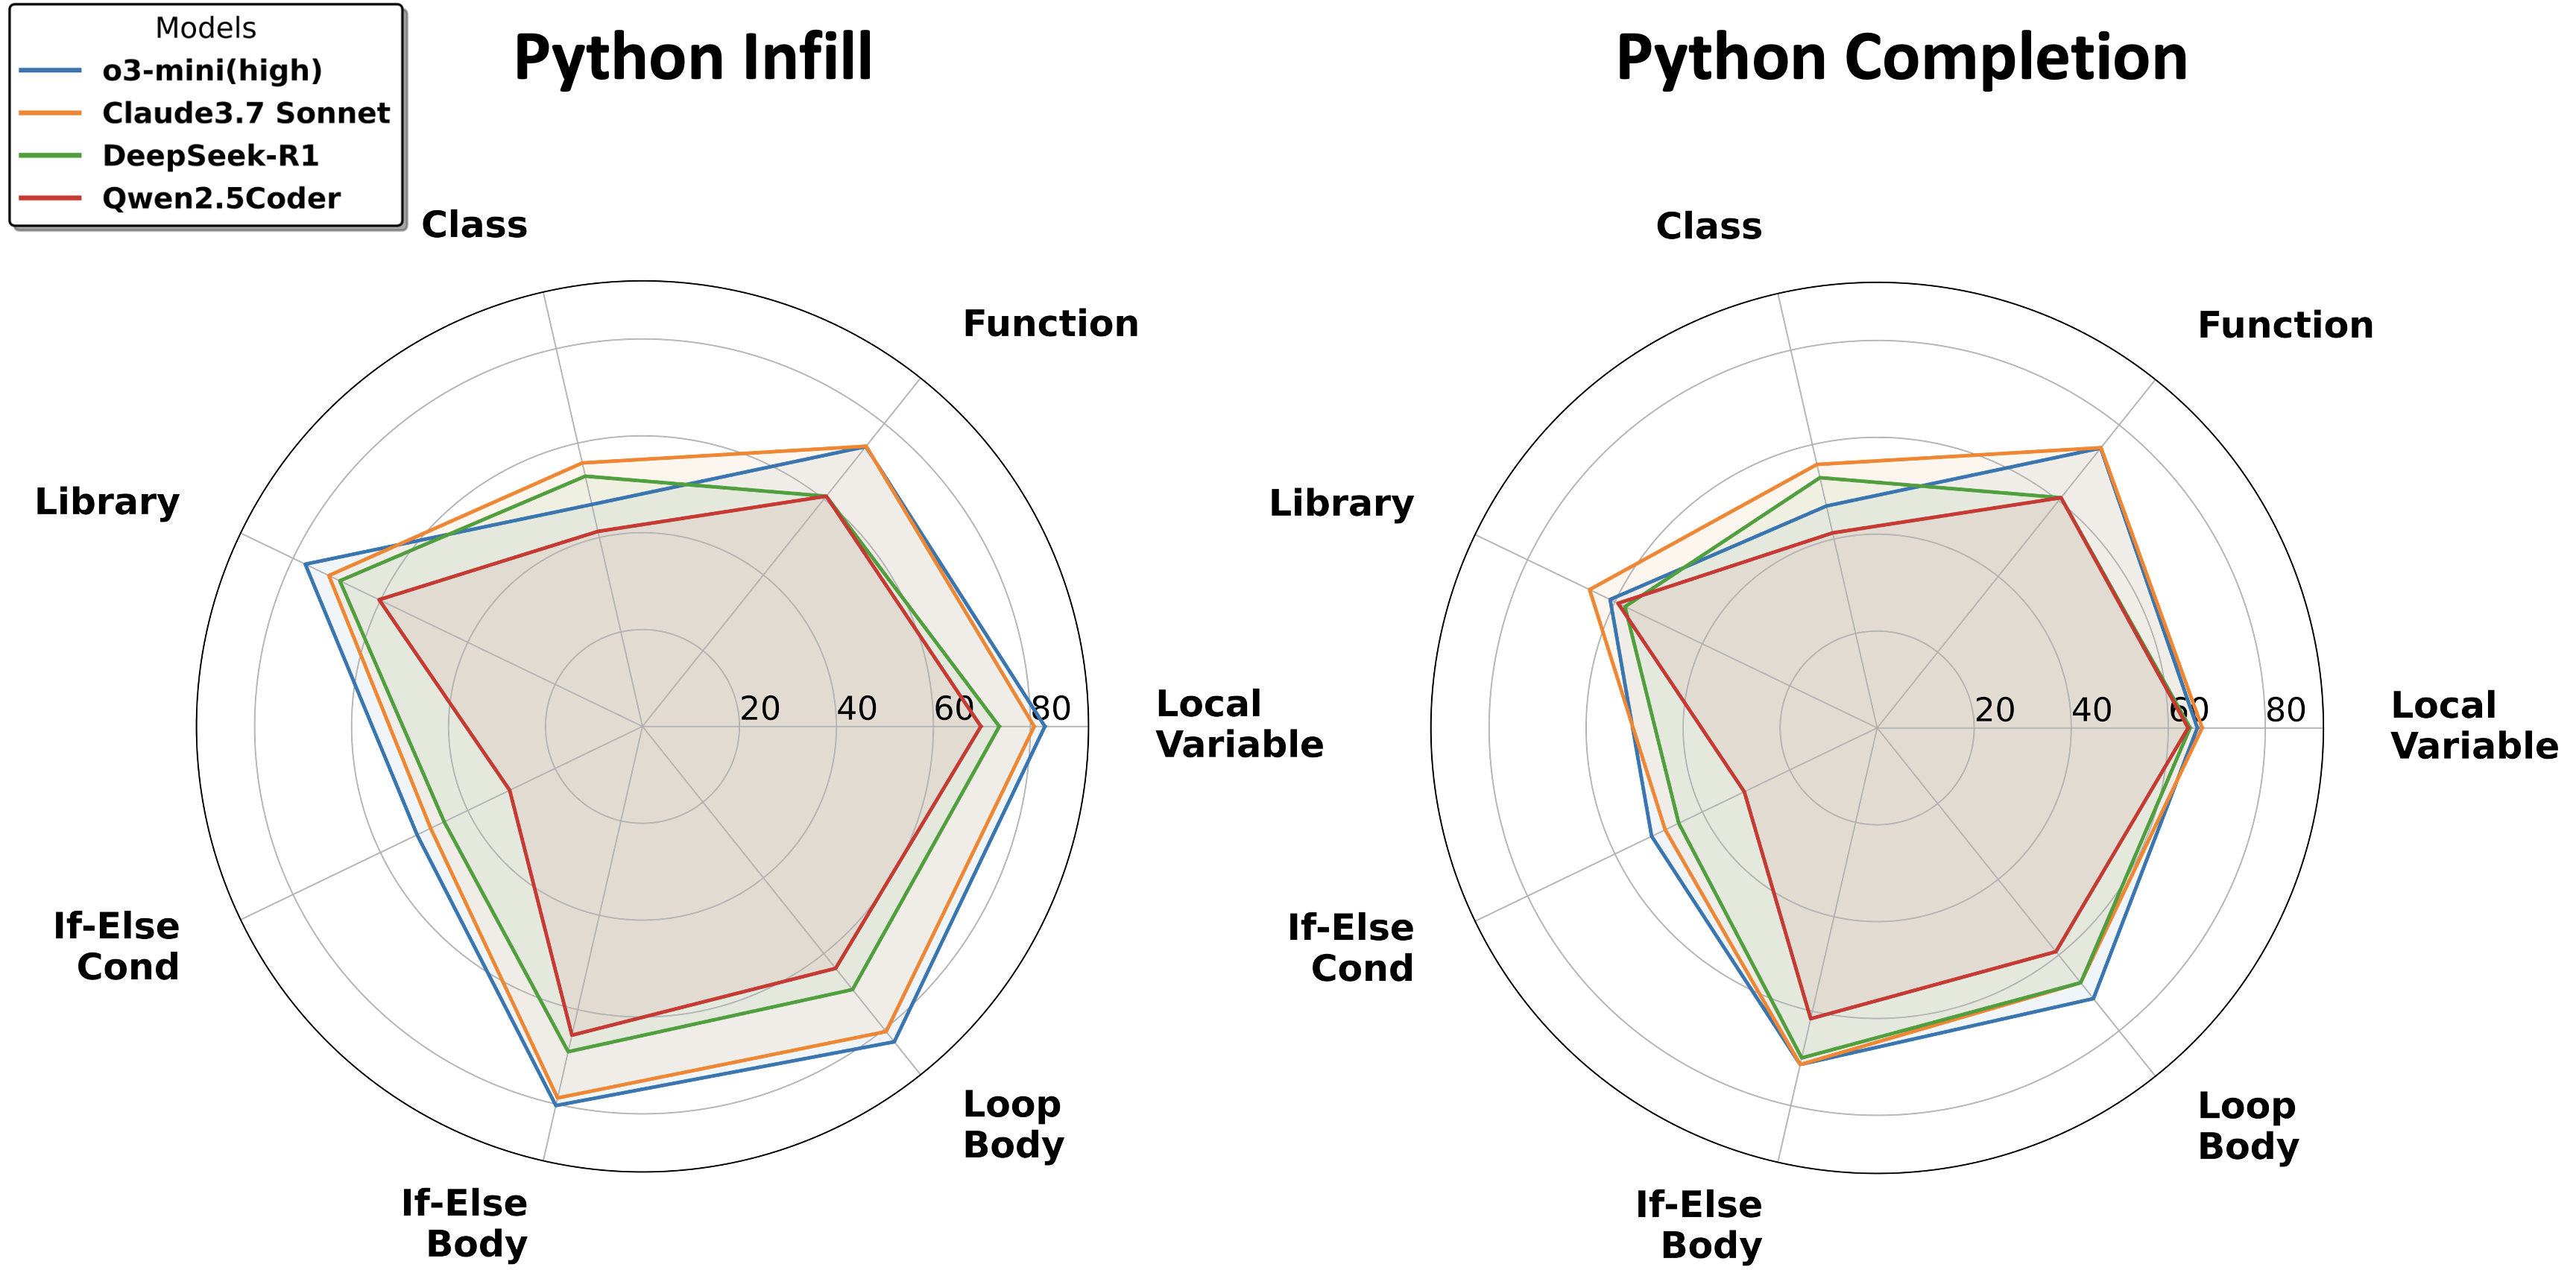}
	\caption{Python Construct}
	\label{fig:python_construct}
\end{figure}

\begin{figure}[h!]
	\centering
	\includegraphics[width= \textwidth]{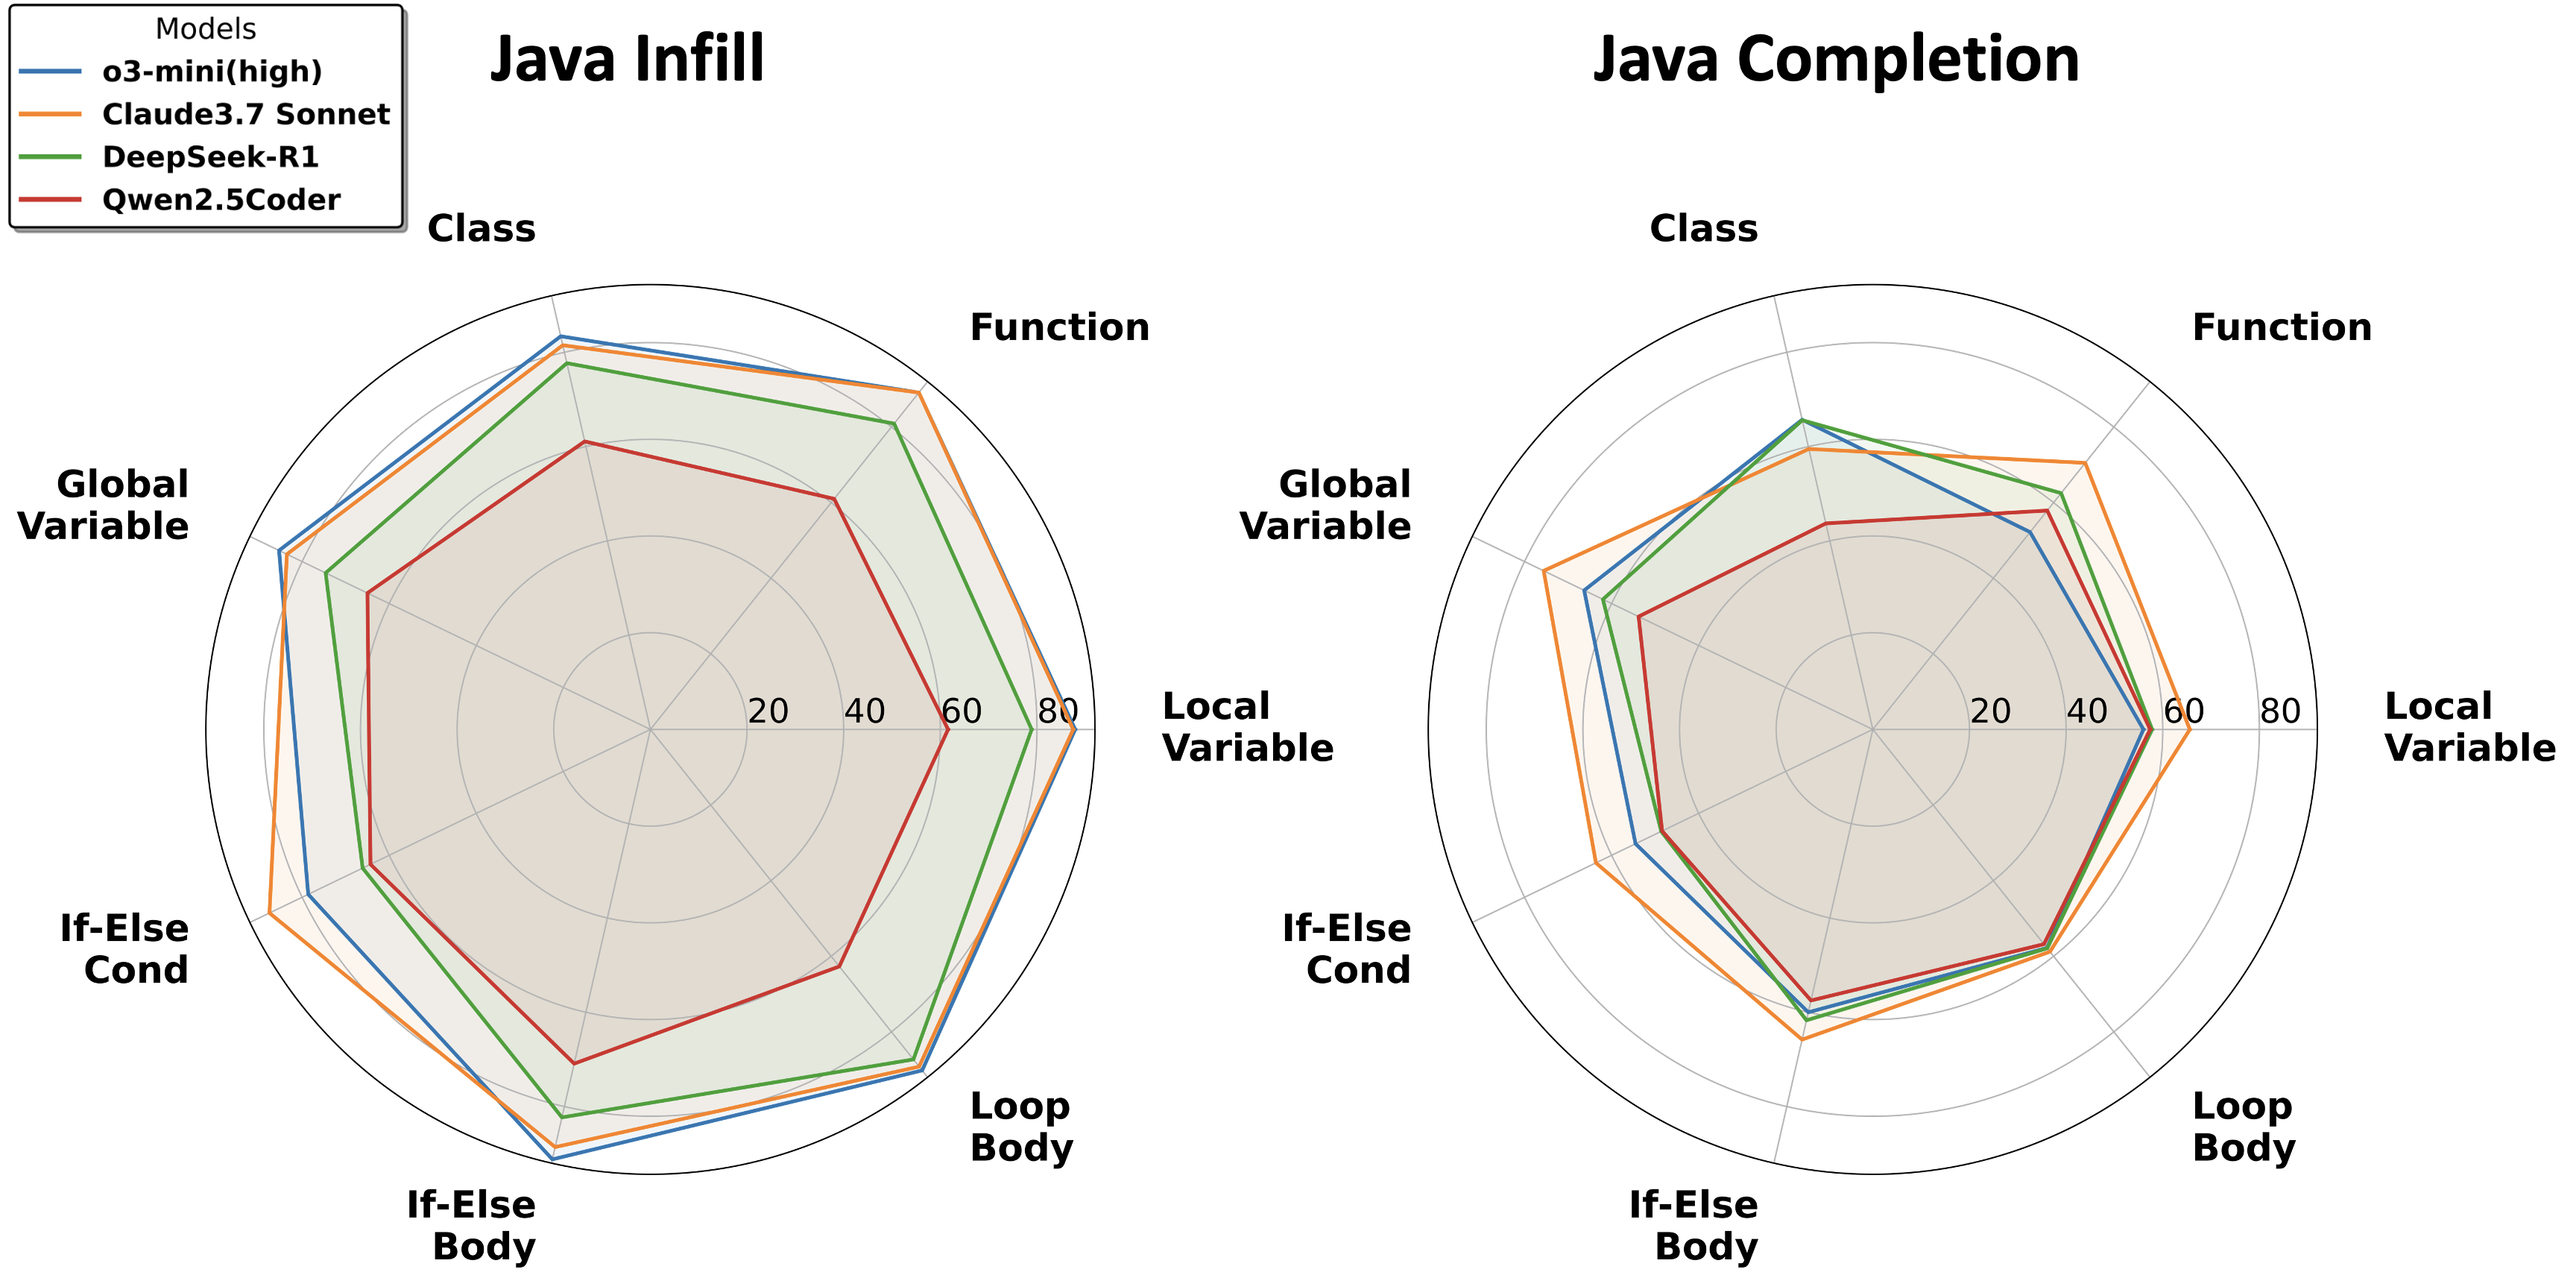}
	\caption{Java Construct}
	\label{fig:java_construct}
\end{figure}
